# Supplementary material for: In Search of Effectful Dependent Types
Source: arXiv:1706.07997 source file (2017-12-06)
Supplement: Supplementary file 1 [file appendix-1.tex]

\begin{savequote}[8cm]

\end{savequote}

\chapter{\label{app:1-papers}Papers}
Please find attached as appendices the written work by the author so far, as part of his DPhil. This constitutes references \cite{vakar2014syntax,vakar2015syntax,abramsky2015games,vakar2016gamsem,vakar2015framework,vakar2016effectful}
. The author would like to stress that while \cite{vakar2015framework,vakar2016effectful} contain the suggestion that the subject reduction property for dCBPV+ with reading and/or writing can be recovered by imposing a subtyping condition, it has since been pointed out to the author that this solution is not satisfactory in the presence of $\Pi$-types.
